# Supplementary material for: Groomed Event Shapes at HERA and the sPHENIX TPC
Source: arXiv:2409.06876 source file (2024-09-10)
Supplement: Supplementary file 1 [file appendix.tex]

\appendix
\chapter{Final Construction}
All the subcomponents mentioned in Chapter~\ref{Chap:TPC} were assembled into the completed TPC in late 2022. The assembly took place largely inside the clean tent at SBU, with the exception of the electronics and the laser systems. The TPC was constructed vertically to remove gravitational deformation from the field cages. The outer field cage in particular is susceptible to deformation, in spite of the aluminum end rings, due to its large size. To aid in the assembly procedure, a large steel structure known as the assembly frame was erected in the tent. The order of operations for the final assembly was as follows: To minimize the time the GEMs were outside the laminar flow tables, the field cages were prepared in their final concentric orientation in advance. Then half the readout modules were mounted to one of the wagon wheels, which was raised and bolted to the assembly frame. \par 
After both field cages were complete, a crane was used to place the outer field cage vertically on a table constructed out of 80-20 and hydraulic legs. The hydraulic table had the ability to be raised by around 3 feet, enable the field cages to be brought up to meet the wagon wheel which was to be hanging from the assembly frame. The table also had wheels, to allow it to roll smoothly into the clean tent. With the outer field cage vertical, it could be accessed from the inside. On the inside of the outer field cage, a variety of operations had to be performed. One of these operations was to epoxy a set of "jumper" copper stripes over an exposed layer of insulator on the striped circuit cards. These jumper stripes then had to be soldered to the main stripes to achieve the proper voltage. 
\begin{figure}[htbp]
    \centering
    \includegraphics[width=6cm]{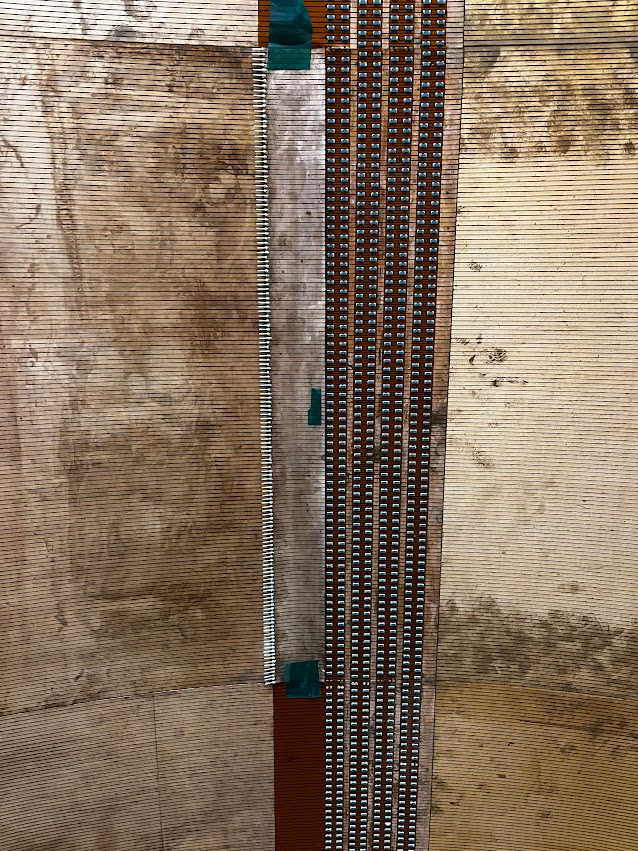}
    \caption{The jumper board covering the exposed insulator. The uncovered insulator can be seen above and below the jumper board. Small wires were soldered between the main field stripes and the jumper stripes to maintain the same voltage.}
    \label{fig:Jumpers}
\end{figure} After this, the field cage was cleaned extensively, and exposed non-conducting surfaces which could potentially outgas were covered with a thin layer of epoxy. The mounting points for the central cathode, whose holders had been placed precisely by microscope, were epoxied into the holders. \par
The next step was to insert the inner field cage into the outer field cage. This was achieved with the overhead crane. With the IFC placed inside the OFC, an alignment procedure brought the two into close concentricity.
